# Supplementary material for: Event-guided Multi-patch Network with Self-supervision for Non-uniform Motion Deblurring
Source: arXiv:2302.07689 source file (2023-02-14)
Supplement: Supplementary file 1 [file appendix.tex]

\section{Outputs of Stacked Network}

Below we present the intermediate outputs of our Stack-VMPHN. Figure \ref{fig:svdnet_comp} shows that the performance is optimized level by level, which is consistent with the behaviour of Stack-DMPHN. We also provide more instances for Stack-DMPHN to demonstrate its process in Figure \ref{fig:supp_comp}.

\begin{figure}[h]
	\vspace{-0.1cm}
	\centering
	\includegraphics[width=\linewidth]{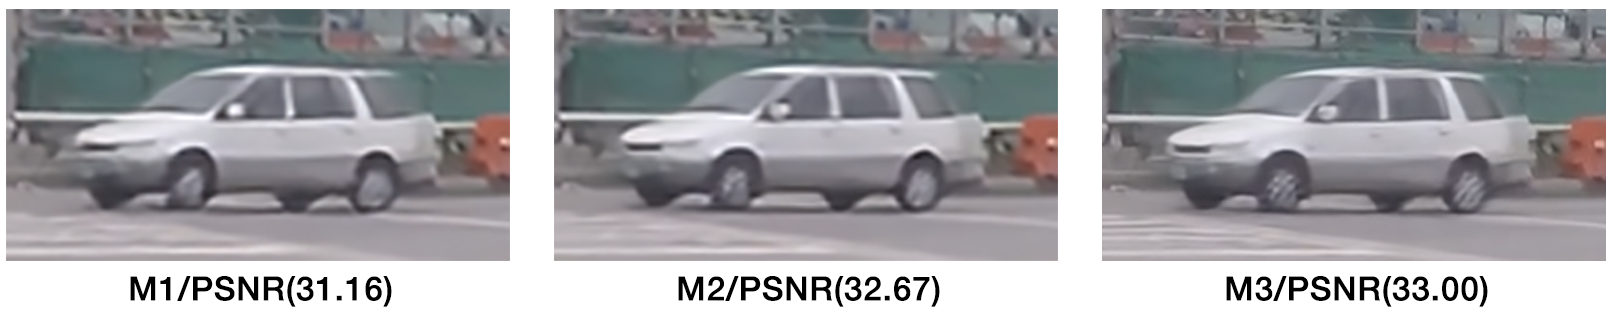}
    \caption{\small The outputs for different sub-models of Stack(3)-VMHPN. From left to right are the outputs of $\mathbf{M}_1$ to $\mathbf{M}_3$.}
	\label{fig:svdnet_comp}
    \vspace{-0.3cm}
\end{figure}

\begin{figure}[h]
	\vspace{-0.4cm}
	\centering
	\includegraphics[width=\linewidth]{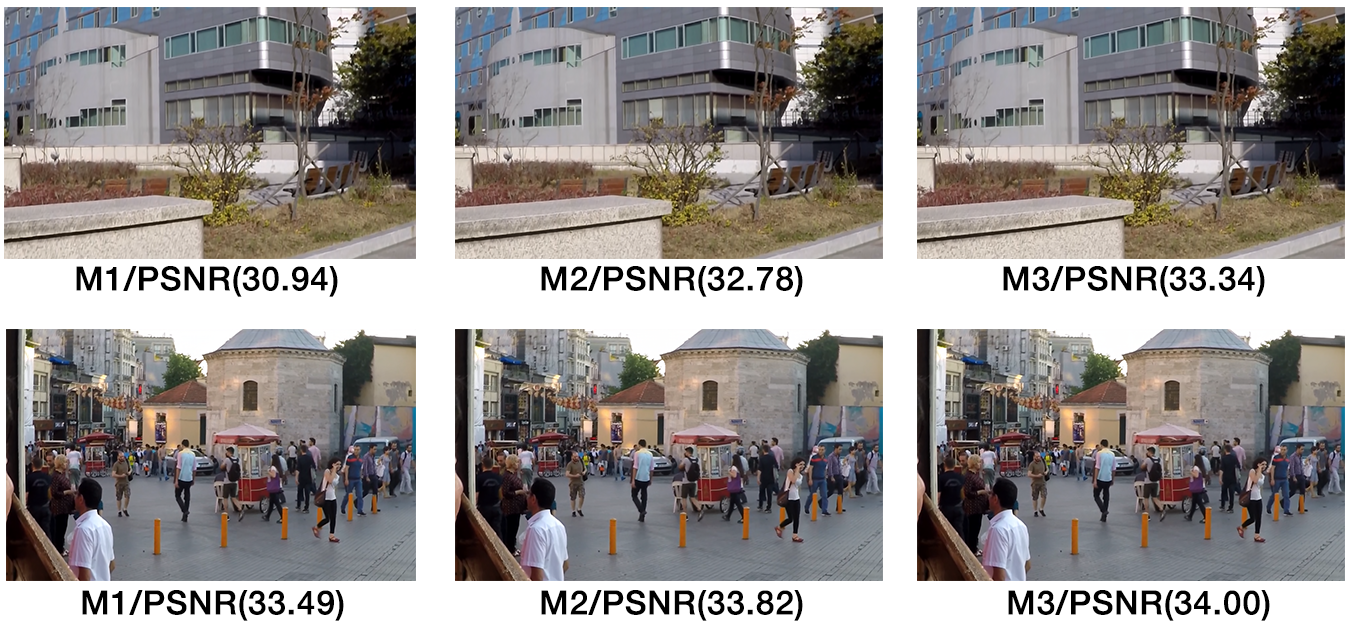}
    \caption{\small The outputs for different sub-models of Stack(3)-DMHPN. From left to right are the outputs of $\mathbf{M}_1$ to $\mathbf{M}_3$.}
	\label{fig:supp_comp}
    \vspace{-0.5cm}
\end{figure}

\section{Extension to Saliency Detection}
\begin{figure}[t]
    \vspace{-0.5cm}
    \centering
    \includegraphics[height=4.5cm]{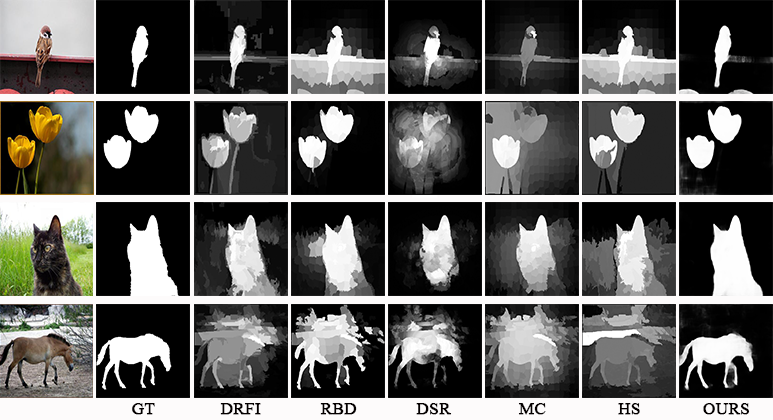}
    \caption{Instances of saliency detection on the MSRA-B dataset.}
    \label{fig:saliency_comp}
    \vspace{-0.3cm}
\end{figure}

%===========================================================
We perform saliency detection with our proposed model to investigate the generalization ability on different tasks. Our proposed model is evaluated on the MSRA-B dataset. This dataset consists of 3000 images for training and 2000 images for testing. Note that all current deep methods of saliency detection highly depend on VGG or ResNet pre-trained on ImageNet and these methods often will not converge without pre-training on ImageNet. By contrast, our network can be easily trained from scratch. It outperforms all conventional methods and it is real-time. We evaluated single VMPHN for quantitative analysis. To make our network compatible with the saliency detection task, the output channel is modified to 1 for gray image generation, and the residual connection between input and output at level 1 is disabled in VMPHN. Figure \ref{fig:saliency_comp} and Table \ref{tabel:share_weight} show our results.

\begin{table}[h]
\caption{\small Quantitative analysis of saliency detection on MSRA-B. For $F_{\beta}$, higher scores are better. For MAE, lower scores are better.}
\makebox{\begin{tabular}{|l|c|c|c|c|c|c|}
\hline
\small Model & \small \cite{jiang2013salient}&\small \cite{zhu2014saliency} &\small \cite{li2013saliency} &\small \cite{jiang2013saliency} &\small \cite{zou2015harf} &\small OURS \\ \hline
\small $F_{\beta}$ & .728 & .751 & .723 & .717 & .713 & \textbf{.768}\\
\small{MAE} & .123 & .117 & .121 & .144 & .161 & \textbf{.107}\\ \hline
\end{tabular}}
\label{tabel:share_weight}
\vspace{-0.4cm}
\end{table}
